# Supplementary material for: Dynamic orders of a Quantum Spin Liquid at Non-zero Temperatures
Source: arXiv:2412.10542 source file (2024-12-13)
Supplement: Supplementary file 1 [file Supplementary-material_Final.pdf]

# Supplemental Material for "Dynamic Orders of Quantum Spin Liquids at non-zero Temperatures"

## I. Connection between QMC results and zero temperature parton analysis

We demonstrate that our QMC results are adiabatically connected to the parton analysis at zero temperature. Namely, the peak around $\omega/(3J) \sim 0.11$ in Fig. 2(c) is smoothly connected to the one of Fig. 4(b) in the main-text. We perform the parton analysis at zero temperature for small number of $N(= 5, 6, 7, 8, \cdots)$ as shown in Fig. S1. The lowest-energy flux sector is determined from 8 different topological sectors for the periodic boundary condition, where all local $\langle W_p \rangle = 1$.

It is clear that the four graphs for $N = 5, 6, 7, 8$ are clearly consistent with the QMC result (blue) for $N = 4$ with parallel tempering [1] in Fig. S1.

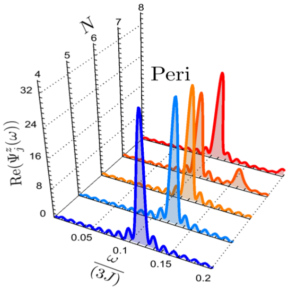


FIG. S1. Comparison with parton analysis at zero temperature ($N = 5, 6, 7, 8$) and QMC results ($N = 4$) at $T = 0.9T_w$. We use $\eta = 0.003$ for $N = 4$ QMC results.

## II. Properties of $D_z$

In this section, we discuss properties of the time averaged local spin correlation function, $D_z$, defined as

$$D_z \equiv \lim_{T_0 \to \infty} \frac{1}{T_0} \int_0^{T_0} dt \, \langle S_j^z(t) S_j^z(0) \rangle. \tag{1}$$

Let us first consider a magnetically ordered phase which has a non-zero expectation value of a local spin operator, $S_j^\alpha(t)$ with $\alpha = x, y, z$. Without loss of generality, one can choose its spin direction as the $z$ direction, giving $m_j \equiv \langle \hat{S}_j^z(t) \rangle > 0$. Then, the $z$ component spin operator can be rewritten as

$$\hat{S}_j^z(t) = m_j \hat{\mathbb{I}} + \delta \hat{S}_j^z(t), \quad \langle \delta \hat{S}_j^z(t) \rangle = 0, \tag{2}$$

where the hat notation $\hat{()}$ is used to notify quantum operators. It is natural to assume that the stability of the ordered phase guarantees small fluctuation in the sense that $\epsilon(t) \equiv ||\delta \hat{S}_j^z(t)||/m_j \ll 1$, where the norm of $\delta \hat{S}_j^z(t)$ can be defined as $||\delta \hat{S}_j^z(t)|| = \sqrt{|\langle \delta \hat{S}_j^z(t) \delta \hat{S}_j^z(0) \rangle|}$, for example. Then, the time averaged local spin correlation function becomes

$$D_z \;=\; m_j^2 \big(1 + \lim_{T_0 \to \infty} \frac{1}{T_0} \int_0^{T_0} dt \frac{\langle \delta \hat{S}_j^z(t) \delta \hat{S}_j^z(0) \rangle}{m_j^2} \big) \geq m_j^2 \big(1 - \lim_{T_0 \to \infty} \frac{1}{T_0} \int_0^{T_0} dt \, \epsilon(t)^2 \big) > 0. \tag{3}$$

Note that $\epsilon(t)$ describes an exponential decay form in usual magnetically ordered phases. Thus, we show that $D_z \neq 0$ for a magnetically ordered phase. Then, its contrapositive is that a magnetically symmetric phase has $D_z = 0$.

## III. Solving sign ambiguity

In this section, we determine the sign of $\sqrt{\det(1 + e^{-(\beta - it)iA} e^{-itiA'})}$. In this case, since $e^A$ is not in the form of a skew-symmetric matrix, the direct application of the robledo formula is challenging [2]. Instead, we use the formula

below, applicable when $H$ is a Hamiltonian of free Majorana fermions. (See appendix A in [3])

$$\mathrm{Tr}[e^{-H}a_{i1}\dots a_{in}a^\dagger_{j1}\dots a^\dagger_{jn}] = D(-H)\times \mathrm{Pf}\begin{pmatrix} 0 & -B_{i_1,i_2} & \cdots & -B_{i_1,i_n} & A_{i_1,j_1} & A_{i_1,j_2} & \cdots & A_{i_1,j_n} \\ -B_{i_2,i_1} & 0 & \cdots & -B_{i_2,i_n} & A_{i_2,j_1} & A_{i_2,j_2} & \cdots & A_{i_2,j_n} \\ \vdots & \vdots & \ddots & \vdots & \vdots & \vdots & \ddots & \vdots \\ -B_{i_n,i_1} & -B_{i_n,i_2} & \cdots & 0 & A_{i_n,j_1} & A_{i_n,j_2} & \cdots & A_{i_n,j_n} \\ A_{j_1,i_1} & A_{j_1,i_2} & \cdots & A_{j_1,i_n} & 0 & -C_{j_1,j_2} & \cdots & -C_{j_1,j_n} \\ A_{j_2,i_1} & A_{j_2,i_2} & \cdots & A_{j_2,i_n} & -C_{j_2,j_1} & 0 & \cdots & -C_{j_2,j_n} \\ \vdots & \vdots & \ddots & \vdots & \vdots & \vdots & \ddots & \vdots \\ A_{j_m,i_1} & A_{j_m,i_2} & \cdots & A_{j_m,i_n} & -C_{j_n,j_1} & -C_{j_n,j_2} & \cdots & 0 \end{pmatrix} \quad (4)$$

$$= D(-H)\times Pf(\hat{S}(-H)) \quad (5)$$

Here, $D(H)$ corresponds to the partition function of $H$, and the matrix $\hat{S}(H)$ is a matrix whose components consist of the Green function of $H$. (Specifically, $A_{ij} = \langle e^{-H}a_i a^\dagger_j\rangle/D$, $B_{ij} = \langle e^{-H}a_i a_j\rangle/D$, and $C_{ij} = \langle e^{-H}a^\dagger_i a^\dagger_j\rangle/D$). Let $H_0 = \sum_{ik}\frac{i}{4}c_i A_{ik}c_k$ and $H' = \sum_{ik}\frac{i}{4}c_i A'_{ik}c_k$. Given that $\langle M_0|$ represents the ground state of $H$, $E_g$ is the ground energy of $H$, and $a$ is the annihilation operator that diagonalizes $H$. Consider the following two equations:

$$\langle M_0|e^{-(\beta-it)H_0}e^{-itH'}|M_0\rangle = e^{-(\beta-it)E_g}\mathrm{Tr}[e^{-itH'}a_1\dots a_N a^\dagger_1\dots a^\dagger_N] \quad (6)$$

$$= e^{-(\beta-it)E_g}D(-itH')Pf(\hat{S}(-itH')) \quad (7)$$

In this case, $D(-itH') = \mathrm{Tr}(e^{-itH'}) = \prod_i 2\cos\frac{t\epsilon_i}{2}$, where $\epsilon_i$ are all the positive eigenvalues of the matrix $A_{j,\alpha}$. Therefore, equation (7) provides an exact value without any sign ambiguity. Meanwhile,

$$\langle M_0|e^{-(\beta-it)H_0}e^{-itH'}|M_0\rangle = \mathrm{Tr}[e^{-(\beta-it)H_0}e^{-itH'}a_1\dots a_N a^\dagger_1\dots a^\dagger_N] \quad (8)$$

$$= D(-(\beta-it)H_0, -itH')Pf(\hat{S}(-(\beta-it)H_0, -itH')) \quad (9)$$

In this case, $D(-(\beta-it)H_0, -itH') = \sqrt{\det(1+e^{-(\beta-it)iA}e^{-itiA'})}$ is the partition function of $e^{-(\beta-it)H_0}e^{-itH'}$ that may have a sign ambiguity. Moreover, $\hat{S}$ can be easily calculated using the following matrix:

$$\begin{pmatrix} a_1 \\ a_2 \\ \vdots \\ a^\dagger_N \end{pmatrix} = \hat{X}\begin{pmatrix} c_1 \\ c_2 \\ \vdots \\ c_{2N} \end{pmatrix} \quad (10)$$

$$\hat{S}(-(\beta-it)H_0, -itH') = \hat{X}[\frac{1}{1+e^{-(\beta-it)iA}e^{-itiA'}}]\hat{X}^\tau \quad (11)$$

Furthermore, by comparing the following expression, a similar method yields $\mathrm{Tr}[(-1)^F e^{-(\beta-it)H_0}e^{-itH'}] = \det(Q)\times\sqrt{\det(1-e^{-(\beta-it)iA}e^{-itiA'})}$ [4]. Given that $\langle M_0|$ is in the vacuum state, which is in the even sector, $(-1)^{F_\gamma} = 1$. Therefore,

$$\langle M_0|(-1)^F e^{-(\beta-it)H_0}e^{-itH'}|M_0\rangle = \det Q\times e^{-(\beta-it)E_g}\mathrm{Tr}[e^{-itH'}a_1\dots a_N a^\dagger_1\dots a^\dagger_N] \quad (12)$$

$$= \det(Q)\times e^{-(\beta-it)E_g}D(-itH')Pf(\hat{S}(-itH')) \quad (13)$$

$$= \det(Q)\times\sqrt{\det(1-e^{-(\beta-it)iA}e^{-itiA'})}Pf(\hat{X}[\frac{1}{1-e^{-(\beta-it)iA}e^{-itiA'}}]\hat{X}^\tau) \quad (14)$$

Using the above method, we have calculated the correlation function and confirmed that it provides the same sign as the results obtained continuously from $t=0$ in all cases. Therefore, we can compute the spin correlation in parallel, which gives us a time advantage. Also, for the N=5 open boundary, our method can be applicable though the previous method in literature might produce the negative sign.

## IV. Correlation function expression for QMC

For the semi-open boundary condition, the Hamiltonian is

$$H = -iJ_x \sum_{\text{x bond}} c_b c_w - iJ_y \sum_{\text{y bond}} c_b c_w - iJ_z \sum_{\text{z bond}} \mu_r c_b c_w \tag{15}$$

Fixing $\mu_r = i\bar{c}_b\bar{c}_w$, we can express the Hamiltonian $H(\mu_r) = \sum_{i,j} \frac{i}{4} c_i A_{ij}(\mu_r) c_j = \frac{i}{4}\mathbf{c}^\tau \hat{A}(\mu_r)\mathbf{c}$. Also, $H'_{j,xy}$ is the Hamiltonian which has different sign for the x,y bonds connected to the j compared to $H$. Additionally, $A'_{j,xy}(\mu_r)$ is the matrix that is identical to $A(\mu_r)$ except the signs for the x and y bonds connected to site j. Let's denote the $\hat{A}(\mu_r) \to \hat{A}$,

$$\langle S^z_j(t) S^z_{j'}(0)\rangle = \frac{1}{4}\frac{\text{Tr}(e^{-\beta H} e^{itH}\sigma^z_j(0) e^{-itH}\sigma^z_{j'}(0))}{\text{Tr}(e^{-\beta H})} = \frac{1}{4}\frac{\text{Tr}(e^{-\beta H} e^{itH} e^{-itH'_{j,xy}}\sigma^z_j(0)\sigma^z_{j'}(0))}{\text{Tr}(e^{-\beta H})} \tag{16}$$

$$= -\frac{1}{4}\frac{\text{Tr}_{\{\mu_r\}}\text{Tr}_{\{c\}}(e^{-(\beta-it)\frac{i}{4}\mathbf{c}^\tau\hat{A}\mathbf{c}} e^{-it\frac{i}{4}\mathbf{c}^\tau\hat{A}'_{j,xy}\mathbf{c}}\bar{c}_j c_j \bar{c}_{j'} c_{j'})}{\text{Tr}_{\{\mu_r\}}\text{Tr}_{\{c\}}(e^{-\beta\frac{i}{4}\mathbf{c}^\tau\hat{A}\mathbf{c}})} \tag{17}$$

$$= \begin{cases} \frac{1}{4}\frac{\text{Tr}_{\{\mu_r\}}\text{Tr}_{\{c\}}(e^{-(\beta-it)\frac{i}{4}\mathbf{c}^\tau\hat{A}\mathbf{c}} e^{-it\frac{i}{4}\mathbf{c}^\tau\hat{A}'_{j,xy}\mathbf{c}})}{\text{Tr}_{\{\mu_r\}}\text{Tr}_{\{c\}}(e^{-\beta\frac{i}{4}\mathbf{c}^\tau\hat{A}\mathbf{c}})} & \text{if } j = j' \\ -\frac{i}{4}\frac{\text{Tr}_{\{\mu_r\}}\text{Tr}_{\{c\}}(e^{-(\beta-it)\frac{i}{4}\mathbf{c}^\tau\hat{A}\mathbf{c}} e^{-it\frac{i}{4}\mathbf{c}^\tau\hat{A}'_{j,xy}\mathbf{c}}\mu_r^{jj'} c_j c_{j'})}{\text{Tr}_{\{\mu_r\}}\text{Tr}_{\{c\}}(e^{-\beta\frac{i}{4}\mathbf{c}^\tau\hat{A}\mathbf{c}})} & \text{if } j - j' \text{ is z bond in Kitaev model} \end{cases} \tag{18}$$

For other case of $j, j'$ sites, $\bar{c}_j$ lead to a different $\{\mu_r\}$ sector, so it is zero under $\text{Tr}_{\{\mu_r\}}$. Ultimately, by using the equation from the following paper [21] and summing over the Majorana fermion contribution,

$$\langle S^z_j(t) S^z_{j'}(0)\rangle = \frac{1}{\text{Tr}_{\{\mu_r\}}\sqrt{(\det(1+e^{-\beta i\hat{A}}))}} \tag{19}$$

$$\times \begin{cases} \frac{1}{4}\text{Tr}_{\{\mu_r\}}\sqrt{\det(1+e^{-(\beta-it)i\hat{A}}e^{-iti\hat{A}'_{j,xy}})} & \text{if } j = j' \\ -\frac{i}{2}\text{Tr}_{\{\mu_r\}}\sqrt{(\det(1+e^{-(\beta-it)i\hat{A}}e^{-iti\hat{A}'_{j,xy}})} \times [\frac{1}{1+e^{-(\beta-it)i\hat{A}}e^{-iti\hat{A}'_{j,xy}}}]_{jj'} \times \mu_r^{jj'}) & \text{if } j - j' = \text{z bond} \end{cases} \tag{20}$$

The advantage of this derivation is that it allows for easy calculation of correlations in the x and y components. Given that $A(\mu_r)_{j,\alpha}$ is the identical matrix $A'(\mu_r)$ except the sign for the bonds other than $\alpha$ bond at j site, it follows that.

$$\langle S^\alpha_j(t) S^\alpha_{j'}(0)\rangle = \frac{1}{\text{Tr}_{\{\mu_r\}}\sqrt{\det(1+e^{-\beta i\hat{A}})}} \tag{21}$$

$$\times \begin{cases} \frac{1}{4}\text{Tr}_{\{\mu_r\}}\sqrt{\det(1+e^{-(\beta-it)i\hat{A}}e^{-iti\hat{A}_{j,\alpha}})} & \text{if } j = j' \\ -\frac{i}{2}\text{Tr}_{\{\mu_r\}}\sqrt{(\det(1+e^{-(\beta-it)i\hat{A}}e^{-iti\hat{A}_{j,\alpha}})} \times [\frac{1}{1+e^{-(\beta-it)i\hat{A}}e^{-iti\hat{A}_{j,\alpha}}}]_{jj'} & \text{if } j - j' = \alpha \text{ bond} \end{cases} \tag{22}$$

When $j - j' = \alpha$ bond $j = b, j' = w$ where $b$, $w$ are in equation (15) to apply this equation. Other correlation should be zero because they have $\bar{c}_j$ after Jordan-Wigner transformation. Note that the calculation with the periodic boundary condition is discussed in previous literature [4].

## V. Projection operator on hyperhoneycomb lattice

In the pure Kitaev model, applying periodic boundary conditions involves the relation $\sigma^\alpha_i = ib^\alpha_i c_i$, which requires the condition:

$$D_j = b^x_j b^y_j b^z_j c_j = 1 \tag{23}$$

to hold for all sites $j$. This ensures the eigenstates of the actual Kitaev spin liquid are selected using the projector operator:

$$P_p = \prod_j \frac{1+D_j}{2} \tag{24}$$

where $j$ runs over all sites in the Kitaev model. To calculate the expectation value of an operator $\hat{O}$ in a Kitaev spin liquid, the expression $\mathrm{Tr}[P_p\hat{O}]$ is used. For an operator $\hat{O}$ that preserves the flux sector, the following equation can be derived [5]:

$$\mathrm{Tr}_{\{\mu_r\}}\mathrm{Tr}_{\{c\}}[P_p\hat{O}] = \mathrm{Tr}_{\{\mu_r\}}\mathrm{Tr}_{\{c\}}[\frac{1+\prod_j D_j}{2}\hat{O}] = \mathrm{Tr}_{\{\mu_r\}}\mathrm{Tr}_{\{c\}}[P_F\hat{O}] \tag{25}$$

Where, $P_F = \frac{1+\prod_j D_j}{2}$. Now, consider a hyperhoneycomb lattice with $M = 4\times N_1\times N_2\times N_3$, where $M$ is total number of unit cells, and $N_1, N_2$ and $N_3$ are the number of unit cells along the $a_1, a_2$ and $a_3$ directions, respectively, as shown in Fig. S2.

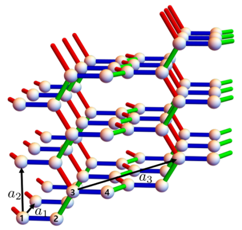


FIG. S2. the graphical representation of the Kitaev model on hyperhoneycomb lattice

Our goal is to express $P_F$ in a form suitable for QMC calculations on the hyperhoneycomb lattice. First, we compute

$$\prod_{j=1}^{M} D_j = \prod_{j=1}^{M} b_j^x b_j^y b_j^z c_j = (i^{\frac{M}{2}}\prod_{j=1}^{M} b_j^x)\times(i^{\frac{M}{2}}\prod_{j=1}^{M} b_j^y)\times(i^{\frac{M}{2}}\prod_{j=1}^{M} b_j^z)\times(i^{\frac{M}{2}}\prod_{j=1}^{M} c_j) \tag{26}$$

The term $i^{\frac{M}{2}}\prod_{j=1}^{M} c_j$ can be expressed as:

$$i^{\frac{M}{2}}\prod_{j=1}^{M} c_j = \prod_{l=1}^{\frac{M}{4}}(ic_{l_1}c_{l_2})(ic_{l_3}c_{l4}) = \prod_{l=1}^{\frac{M}{4}}(1-2f_l^{a\dagger}f_l^a)(1-2f_l^{b\dagger}f_l^b) = (-1)^F \tag{27}$$

where, $l$ runs over $N_1\times N_2\times N_3$ unit cells, and the sublattice index $m\in\{1,2,3,4\}$ is shown in Fig. S2. Here, $c_{l_m}$ represents the Majorana fermion at the $l$-th unit cell and sublattice $m$. The $f$-fermion operators are defined as: $c_{l_1} = i(f_l^{a\dagger}-f_l^a), c_{l_2} = f_l^{a\dagger}+f_k^a$ and $c_{l_3} = i(f_l^{b\dagger}-f_l^b), c_{l_4} = f_l^{b\dagger}+f_l^b$.

For a general free Majorana Hamiltonian,

$$H = \sum_{i,j} ic_iA_{ij}c_j = 2i\sum_m \epsilon_m d'_m d''_m \tag{28}$$

where $\epsilon_m$ are the positive eigenvalues of $iA$ and $d'_m, d''_m$ are another set of Majorana operators. We can find a matrix $\hat{Q}$ such that $(d'_1, d''_1, ..., d'_{\frac{M}{2}}, d''_{\frac{M}{2}}) = (c_1, ..., c_M)\hat{Q}$. It follows that

$$i^{\frac{M}{2}}\prod_{j=1}^{\frac{M}{2}} d'_j d''_j = \det(Q)\times i^{\frac{M}{2}}\prod_{j=1}^{M} c_j = \det(Q)\times(-1)^F. \tag{29}$$

We define $(-1)^{F_\gamma} = i^{\frac{M}{2}} \prod_{j=1}^{\frac{M}{2}} d'_j d''_j$ as fermion parity of the $d$ Marjorana fermions. The $\mathbb{Z}_2$ variable is defined as $u_{ij} = ib^o_i b^e_j$, where, $o$ and $e$ denote sublattice indices corresponding to odd ($o \in \{1,3\}$) and even ($e \in \{2,4\}$) sublattices, respectively. To express the $b^z$ Majorana operator in terms of $u_{ij}$, consider the following:

$$i^{\frac{M}{2}} \prod_{j=1}^{M} b^z_j = \prod_{l=1}^{\frac{M}{4}} (ib^z_{l_1} b^z_{l_2})(ib^z_{l_3} b^z_{l_4}) = \prod_{l=1}^{\frac{M}{4}} u^z_{l_1 l_2} u^z_{l_3 l_4}, \tag{30}$$

where $b^z_{l_m}$ denotes the $b^z$ Majorana operator located at the $m$-th sublattice of the $l$-th unit cell. $u^z_{l_1,l_2}$ is $\mathbb{Z}_2$ variable defined between the sites $l_1$ and $l_2$. $b^x$ and $b^y$ operators can also be expressed in terms of the $u_{ij}$.

In the hyperhoneycomb lattice, the Kitaev Hamiltonian can be viewed as connecting multiple $xy$ chains with $zz$ bonds. Let us define $M_1 = N_1 \times N_3$, $M_2 = N_2 \times N_3$, where $M_1$ and $M_2$ represent the number of $xy$ chains in the $a_2$ and $a_1$ directions, respectively. Each $xy$ chain with the $a_2$ direction is labeled as $s_1$, with sites within them labeled as $p_1$. Here, $p_1$ ranges from 1 to $2N_2$ and increases along the $a_2$ direction. Similarly each $xy$ chain with the $a_1$ direction is labeled as $s_2$, with sites within them labeled as $p_2$. Here, $p_2$ ranges from 1 to $2N_1$ and increases along the $a_1$ direction. Using these definitions, the product of $b^x$ and $b^y$ operators across all sites can be written as:

$$(i^{\frac{M}{2}} \prod_{j=1}^{M} b^x_j)(i^{\frac{M}{2}} \prod_{j=1}^{M} b^y_j) = [i^{\frac{M}{2}} \prod_{s_1=1}^{M_1} (\prod_{p_1=1}^{2N_2} b^x_{s_1,p_1}) \prod_{s_2=1}^{M_2} (\prod_{p_2=1}^{2N_1} b^x_{s_2,p_2})][i^{\frac{M}{2}} \prod_{s_1=1}^{M_1} (\prod_{p_1=1}^{2N_2} b^y_{s_1,p_1}) \prod_{s_2=1}^{M_2} (\prod_{p_2=1}^{2N_1} b^y_{s_2,p_2})] \tag{31}$$

where, $b^{x,y}_{s,p}$ represents the $b^{x,y}$ operator at $p$-th site in the $s$-th $xy$ chain. This equality holds because reordering $b^x$ and $b^y$ in the same manner does not introduce a sign change. For a single chain with $2N$ sites, the product of $b^x$ operators can be expressed as:

$$i^N \prod_{p=1}^{2N} b^x_{s,p} = i^N b^x_{s,1} b^x_{s,2} \dots b^x_{s,2N} = i^N (-1)^{(2N-1)} b^x_{s,2} b^x_{s,3} \dots b^x_{s,2N} b^x_{s,1} = (-1)^{(-1)} \prod_{p=1}^{N} u^x_{(s,2p),(s,2p+1)} \tag{32}$$

Similarly, for $b^y$:

$$i^N \prod_{p=1}^{2N} b^y_{s,p} = i^N b^y_{s,1} b^y_{s,2} \dots b^y_{s,2N} = i^N (-1)^N b^y_{s,2} b^y_{s,1} b^y_{s,4} b^y_{s,3} \dots b^y_{s,2N} b^y_{2N-1} = (-1)^N \prod_{p=1}^{N} u^y_{(s,2p),(s,2p-1)} \tag{33}$$

where, $(s,p)$ is $p$-th site for $s$-th $xy$ chain. $u^{x,y}_{(s,2p),(s,2p+1)}$ represents the $\mathbb{Z}_2$ variable between the sites $(s,2p)$ and $(s,2p+1)$. Substituting the single-chain expressions into the full product, we have:

$$[i^{\frac{M}{2}} \prod_{s_1=1}^{M_1} (\prod_{p_1=1}^{2N_2} b^x_{s_1,p_1}) \prod_{s_2=1}^{M_2} (\prod_{p_2=1}^{2N_1} b^x_{s_2,p_2})][i^{\frac{M}{2}} \prod_{s_1=1}^{M_1} (\prod_{p_1=1}^{2N_2} b^y_{s_1,p_1}) \prod_{s_2=1}^{M_2} (\prod_{p_2=1}^{2N_1} b^y_{s_2,p_2})] \tag{34}$$

$$= (-1)^{M_1 \times (N_2-1) + M_2 \times (N_1 - 1)} [\prod_{s_1=1}^{M_1} (\prod_{p_1=1}^{N_2} u^x_{(s_1,2p_1),(s_1,2p_1+1)} u^y_{(s_1,2p_1),(s_1,2p_1-1)}) \prod_{s_2=1}^{M_2} (\prod_{p_2=1}^{N_1} u^x_{(s_2,2p_2),(s_2,2p_2+1)} u^y_{(s_2,2p_2),(s_2,2p_2-1)})] \tag{35}$$

Consequently, substituting (29), (30), (35) to equation (26) gives

$$P_F = (1 + (\prod_{\alpha=x,y,z} \prod_{i \in A} u^\alpha_i) \times \det(Q) \times (-1)^{F_\gamma})/2 \tag{36}$$

for hyperhoneycomb lattice with $N = N_1 = N_2 = N_3$. Here, $A$ is the set of all sites with odd sublattice indices, and $u^\alpha_i$ is the $\mathbb{Z}_2$ variable in the $\alpha$-direction at site i.

[1] R. H. Swendsen and J.-S. Wang, Physical review letters **57**, 2607 (1986).
[2] L. M. Robledo, Physical Review C—Nuclear Physics **79**, 021302 (2009).
[3] J. Knolle, *Dynamics of a Quantum Spin Liquid* (Springer, 2016).
[4] M. Udagawa, Journal of Physics: Condensed Matter **33**, 254001 (2021).
[5] F. L. Pedrocchi, S. Chesi, and D. Loss, Physical Review B—Condensed Matter and Materials Physics **84**, 165414 (2011).
